# Supplementary material for: The conformational phase diagram of charged polymers in the presence of attractive bridging crowders
Source: arXiv:2308.09328 ancillary file (2023-08-18)
Supplement: Supplementary file 1 [file Supp.pdf]

## Supporting Information

# The conformational phase diagram of charged polymers in the presence of attractive bridging crowders

Kamal Tripathi,[1, a] Hitesh Garg,[2, 3, b] R Rajesh,[2, 3, c] and Satyavani Vemparala[2, 3, d]

[1] *Univ. Grenoble Alpes, CNRS, Grenoble INP, 3SR, F-38000 Grenoble, France*

[2] *The Institute of Mathematical Sciences, C.I.T. Campus, Taramani, Chennai 600113, India*

[3] *Homi Bhabha National Institute, Training School Complex, Anushakti Nagar, Mumbai 400094, India*

(Dated: 18 August 2023)

[a] Electronic mail: kamalt@imsc.res.in

[b] Electronic mail: hiteshgarg@imsc.res.in

[c] Electronic mail: rrajesh@imsc.res.in

[d] Electronic mail: vani@imsc.res.in

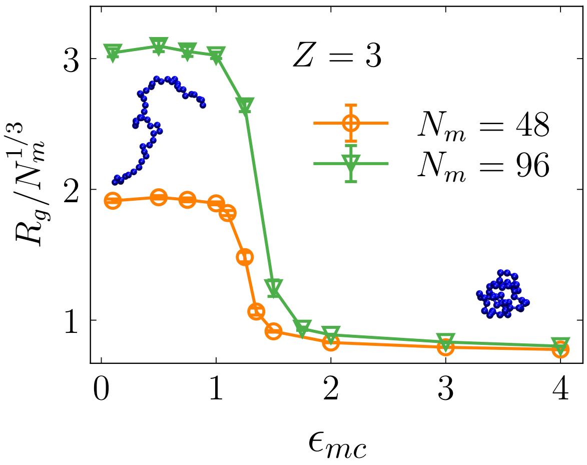


FIG. S1. The scaled $R_g$ for two different $N_m$ is shown for $A/A_c = 0.1$ and $Z = 3$. The snapshots are typical configurations of the PE for $N_m = 48$ for $\epsilon_{mc} = 0.1$ and $\epsilon_{mc} = 3.0$.

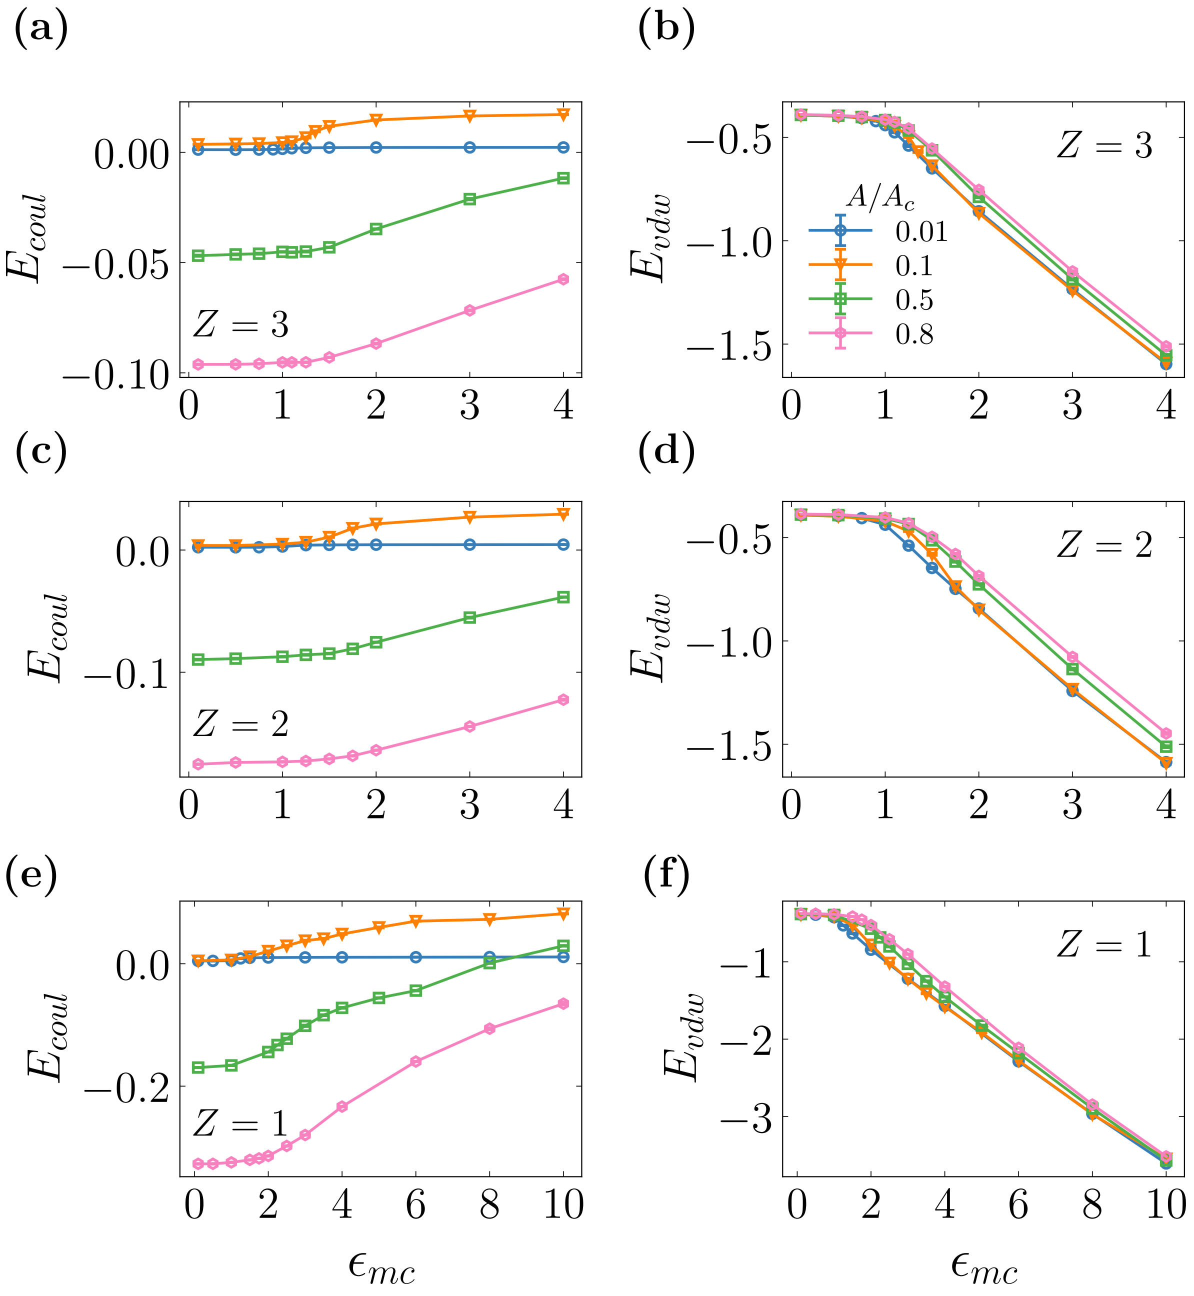


FIG. S2. $A/A_c < 1.0$: The electrostatic energy per particle, $E_{coul}$, and van der Waals energy per particle, $E_{vdw}$ as a function of $\epsilon_{mc}$ for (a, b) $Z = 3$, (c, d) $Z = 2$, (e, f) $Z = 1$.

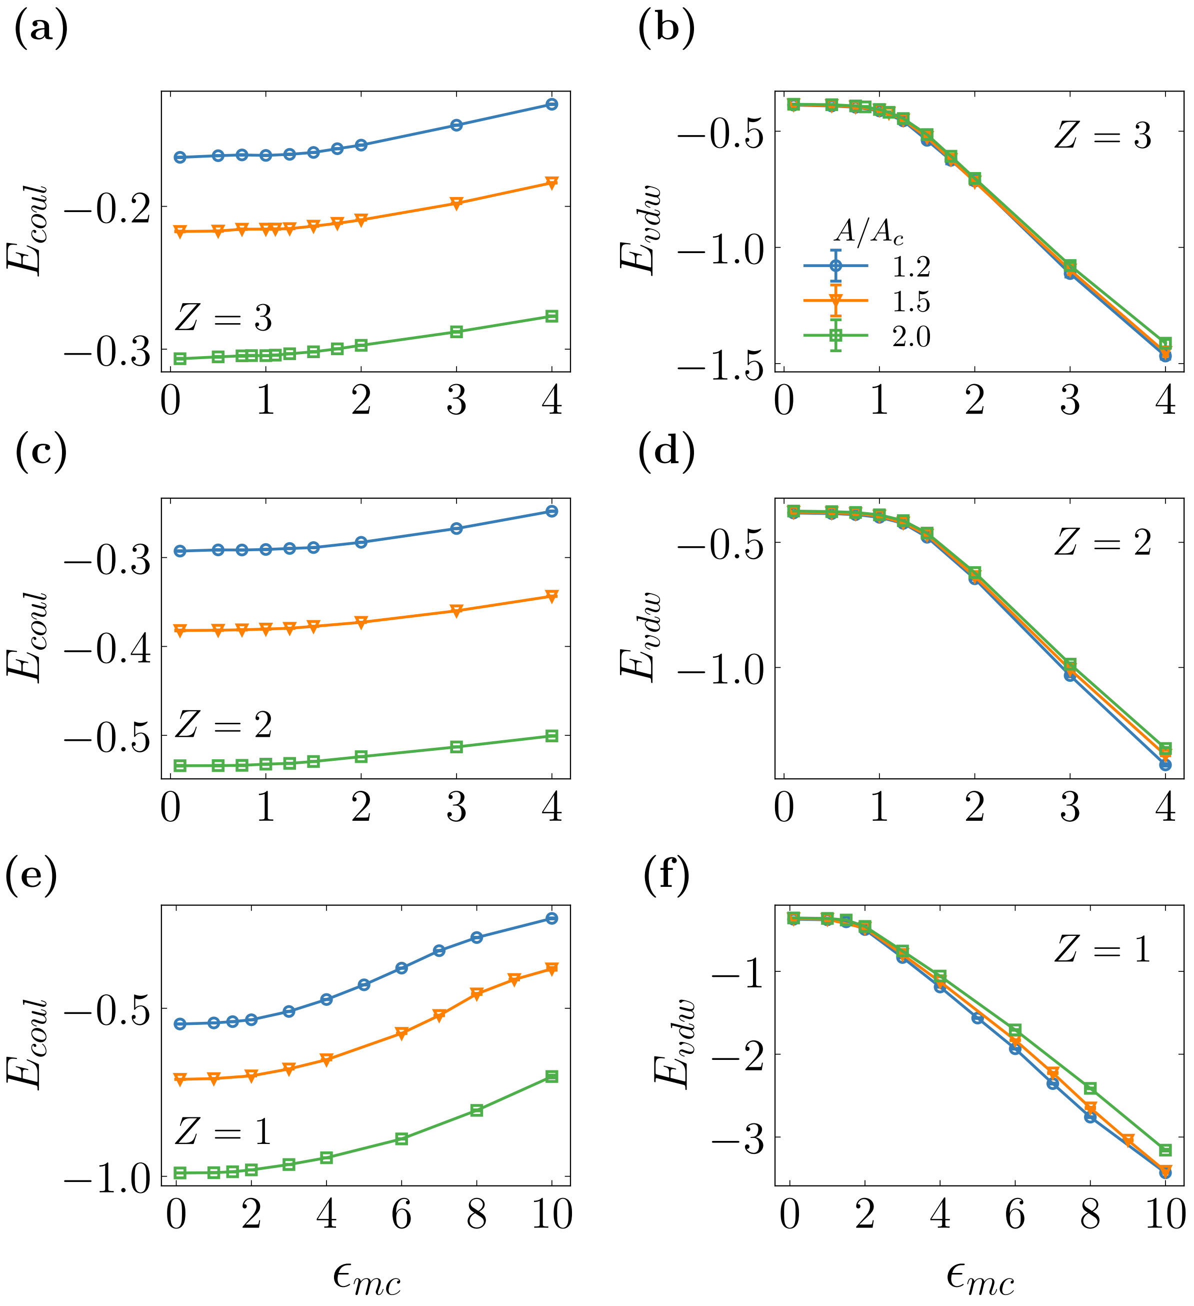


FIG. S3. $A/A_c > 1.0$: The electrostatic energy per particle, $E_{coul}$, and van der Waals energy per particle, $E_{vdw}$ as a function of $\epsilon_{mc}$ for (a, b) $Z = 3$, (c, d) $Z = 2$, (e, f) $Z = 1$.
